# Supplementary material for: BreakingBED -- Breaking Binary and Efficient Deep Neural Networks by Adversarial Attacks
Source: arXiv:2103.08031 source file (2021-03-14)
Supplement: Supplementary file 1 [file 482_StressStrain_supp.tex]

Fig.~\ref{fig:Attack_graphs_supp} shows additional stress-strain graphs for different attacks (a-e) on compressed variants of ResNet20  and ResNet56, as referred to in the paper.

\begin{figure}[b]
\captionsetup[subfigure]{labelformat=empty}
\centering
\subfloat{
\hspace{10ex}
       \input{img/stress_strain_wacv/plot_legend.tex}
} \\\vspace{-2ex}
\subfloat[PGD - Fixed $\epsilon=0.5$ ResNet20]{
       \input{img/stress_strain_wacv/PGD_ResNet20_stress_strain_fixedamp.tex}
       }
\subfloat[LocalSearch - ResNet20 Fixed $\epsilon=16$]{
       \input{img/stress_strain_wacv/LocalSearch_ResNet20_stress_strain.tex}
       }
\subfloat[LocalSearch - ResNet20 Fixed $\epsilon=32$]{
       \input{img/stress_strain_wacv/LocalSearch_ResNet20_e32_stress_strain.tex}
       }
       \\\vspace{-2ex}
\subfloat[PGD - Fixed $\epsilon=0.5$ ResNet56]{
       \input{img/stress_strain_wacv/PGD_ResNet56_stress_strain_fixedamp.tex}
       }
\subfloat[LocalSearch - ResNet56 Fixed $\epsilon=16$]{
       \input{img/stress_strain_wacv/LocalSearch_ResNet56_stress_strain.tex}
       }
\subfloat[LocalSearch - ResNet56 Fixed $\epsilon=32$]{
       \input{img/stress_strain_wacv/LocalSearch_ResNet56_e32_stress_strain.tex}
       }
       \\\vspace{-2ex}
\subfloat[CW - ResNet20 Fixed $\epsilon=1$]{
       \input{img/stress_strain_wacv/CW_ResNet20_stress_strain.tex}
       }
\subfloat[CW - ResNet56 Fixed $\epsilon=1$]{
       \input{img/stress_strain_wacv/GenAttack_ResNet20_e12_stress_strain.tex}
       }\\\vspace{-2ex}
\subfloat[GenAttack - ResNet20 - $\epsilon=8$ $|$ $p=16$]{
       \input{img/stress_strain_wacv/CW_ResNet56_stress_strain.tex}
       }
\subfloat[GenAttack - ResNet56 - $\epsilon=8$ $|$ $p=16$]{
       \input{img/stress_strain_wacv/GenAttack_ResNet56_e12_stress_strain.tex}
       }
\caption{Stress-strain graphs for attacks (a-d) on compressed variants of ResNet20 (Top) and ResNet56 (Bottom).
%\alex{REMOVE: BatchNorm~\cite{bn} layers are in $\mathtt{statistics}$ mode.}
}
\vspace{-1ex}
\label{fig:Attack_graphs_supp}
\end{figure}
