# Supplementary material for: BreakingBED -- Breaking Binary and Efficient Deep Neural Networks by Adversarial Attacks
Source: arXiv:2103.08031 source file (2021-03-14)
Supplement: Supplementary file 3 [file 420_Experiments_PGD_supp.tex]

The adversarial attacks examined w.r.t. PGD are summarized in Tab.~\ref{tab:PGDResnet20_eval}, \ref{tab:PGDResnet56_eval} and \ref{tab:PGDImageNet_eval} for ResNet20, ResNet56 and ImageNet-trained CNNs. 
%Tab.~\ref{tab:PGDResnet20_train}, \ref{tab:PGDResnet56_train} and \ref{tab:PGDImageNet_train} details the results for the BatchNorm's $\mathtt{mini}$-$\mathtt{batch}$ mode. 
PGD is applied for $\epsilon\in \{0.1,0.5,1.0,2.0\}$ multiple iterations $i\in\{2,3,4,5\}$.
