# Supplementary material for: BreakingBED -- Breaking Binary and Efficient Deep Neural Networks by Adversarial Attacks
Source: arXiv:2103.08031 source file (2021-03-14)
Supplement: Supplementary file 9 [file supp_egpaper_for_review.tex]

\documentclass[10pt,twocolumn,letterpaper]{article}
\usepackage[export]{adjustbox}
\usepackage{makecell}
\usepackage{cvpr}
\usepackage{times}
\usepackage{epsfig}
\usepackage{graphicx}
\usepackage{amsmath}
\usepackage{amssymb}
\usepackage{mathtools}
\usepackage{xcolor}
\usepackage{multirow}
\usepackage{subcaption}
\usepackage{booktabs}
\usepackage{amssymb}% http://ctan.org/pkg/amssymb
%red boarder around CAM images
\fboxsep=-.1mm%padding thickness
\fboxrule=0.8pt%border thickness
%
%\usepackage{tikz}
%\usetikzlibrary{shapes.geometric, arrows}

\makeatletter
\@namedef{ver@everyshi.sty}{}
\makeatother
\usepackage{tikz}
\usepackage{pgfplots}
\usepackage{pgfplotstable}

\definecolor{Pal_1}{HTML}{4472C4}
\definecolor{Pal_2}{HTML}{ED7D31}
\definecolor{Pal_3}{HTML}{A5A5A5}
\definecolor{Pal_4}{HTML}{FFC000}
\definecolor{Pal_5}{HTML}{5B9BD5}
\definecolor{Pal_6}{HTML}{70AD47}
\definecolor{Pal_7}{HTML}{264478}
\definecolor{Pal_8}{HTML}{122366}

\pgfplotscreateplotcyclelist{mycolorlist}{%
Pal_1 ,mark=x,mark options={scale=2}\\%
Pal_2,mark=square\\%
Pal_7,mark=square\\%
Pal_4, mark=diamond\\%
Pal_5, mark=triangle\\%
Pal_6,mark=triangle\\%
Pal_3,mark=triangle\\%
Pal_8,mark=triangle\\%
Pal_1 ,mark=o\\%
Pal_2,mark=o\\%
}

\input{misc/happinet_tools.tex}

% Include other packages here, before hyperref.

% If you comment hyperref and then uncomment it, you should delete
% egpaper.aux before re-running latex.  (Or just hit 'q' on the first latex
% run, let it finish, and you should be clear).
\usepackage[pagebackref=true,breaklinks=true,letterpaper=true,colorlinks,bookmarks=false]{hyperref}

% \cvprfinalcopy % *** Uncomment this line for the final submission

\def\cvprPaperID{3} % *** Enter the CVPR Paper ID here
\def\httilde{\mbox{\tt\raisebox{-.5ex}{\symbol{126}}}}

% Pages are numbered in submission mode, and unnumbered in camera-ready
\ifcvprfinal\pagestyle{empty}\fi
\begin{document}

%%%%%%%%% TITLE
\title{Supplementary Material: BreakingBED - Breaking Binary and Efficient Deep Neural Networks by Adversarial Attacks}
\input{misc/authors.tex}

\maketitle
%\thispagestyle{empty}

    
%  ___      __   ___  __           ___      ___  __  
% |__  \_/ |__) |__  |__) |  |\/| |__  |\ |  |  /__` 
% |___ / \ |    |___ |  \ |  |  | |___ | \|  |  .__/ 
\section{Experimental Results}
    \input{data/experiments/40_experimental_setup_supp.tex}
    % %             ___  ___  __   __      
    % % |  | |__| |  |  |__  |__) /  \ \_/ 
    % % |/\| |  | |  |  |___ |__) \__/ / \
    
    \subsection{Adversarial Attacks on FGSM}
    \input{data/experiments/41_FGSM/410_Experiments_FGSM_supp.tex}
    \input{data/experiments/41_FGSM/411_Experiments_FGSM_ResNet20.tex}
    \input{data/experiments/41_FGSM/412_Experiments_FGSM_ResNet56.tex}
    \input{data/experiments/41_FGSM/413_Experiments_FGSM_ImageNet.tex}
    
    \subsection{Adversarial Attacks on PGD}
    \input{data/experiments/42_PGD/420_Experiments_PGD_supp.tex}
    \input{data/experiments/42_PGD/422_Experiments_PGD_ResNet56_eval.tex}
    \input{data/experiments/42_PGD/421_Experiments_PGD_ResNet20_train.tex}
    
    \input{data/experiments/42_PGD/422_Experiments_PGD_ResNet56_train.tex}
    \input{data/experiments/42_PGD/423_Experiments_PGD_ImageNet_train.tex}
    
    
    \subsection{Adversarial Attacks on Carlini \& Wagner}
    \input{data/experiments/43_CW/430_Experiments_CW_supp.tex}
    \input{data/experiments/43_CW/431_Experiments_CW_ResNet20_train.tex}
    \input{data/experiments/43_CW/432_Experiments_CW_ResNet56_eval.tex}
    \input{data/experiments/43_CW/432_Experiments_CW_ResNet56_train.tex}
    
    \subsection{Adversarial Attacks on DeepFool}
    \input{data/experiments/44_DeepFool/440_Experiments_Deepfool.tex}
    \input{data/experiments/44_DeepFool/441_Experiments_Deepfool_ResNet20.tex}
    \input{data/experiments/44_DeepFool/442_Experiments_Deepfool_ResNet56.tex}
    %  __             __        __   __      
    % |__) |     /\  /  ` |__/ |__) /  \ \_/ 
    % |__) |___ /~~\ \__, |  \ |__) \__/ / \
    \subsection{Adversarial Attacks on LocalSearch}
    \input{data/experiments/45_LocalSearch/450_Experiments_LocalSearch_supp.tex}
    \input{data/experiments/45_LocalSearch/451_Experimental_LocalSearch_ResNet20_train.tex}
    \input{data/experiments/45_LocalSearch/452_Experimental_LocalSearch_ResNet56_eval.tex}
    \input{data/experiments/45_LocalSearch/452_Experimental_LocalSearch_ResNet56_train.tex}
    \input{data/experiments/45_LocalSearch/453_Experiments_LocalSearch_ImageNet_train.tex}
    
    
    \subsection{Adversarial Attacks on GenAttack}
    \input{data/experiments/46_GenAttack/460_Experimental_Setup_GenAttack_supp.tex}
    \input{data/experiments/46_GenAttack/461_Experimental_GenAttack_ResNet20_train.tex}
    \input{data/experiments/46_GenAttack/462_Experimental_GenAttack_ResNet56_eval.tex}
    \input{data/experiments/46_GenAttack/462_Experimental_GenAttack_ResNet56_train.tex}
    \input{data/experiments/46_GenAttack/463_Experiments_GenAttack_ImageNet_train.tex}

    \subsection{Class Activation Mapping on Attacked CNNs}
    \input{data/experiments/47_CAM/470_CAM_supp.tex}
    \input{data/experiments/47_CAM/473_CAM_ImageNet.tex}
    



%  __   ___  ___  ___  __   ___       __   ___  __  
% |__) |__  |__  |__  |__) |__  |\ | /  ` |__  /__` 
% |  \ |___ |    |___ |  \ |___ | \| \__, |___ .__/
\clearpage
{\small
\bibliographystyle{ieee_fullname}
\bibliography{references}
}
%\input{misc/todoes.tex}
\end{document}
